# Supplementary material for: What is Fair? Defining Fairness in Machine Learning for Health
Source: arXiv:2406.09307 source file (2025-05-27)
Supplement: Supplementary file 1 [file supplementary.tex]

\documentclass[12pt]{article}

% Package
\usepackage{geometry}
\usepackage[utf8]{inputenc}
\usepackage{authblk}

\usepackage{setspace}
%\usepackage[backend=biber,style=nature, isbn=false,url=false,eprint=false]{biblatex}
%\addbibresource{references.bib}
%\usepackage{natbib}
\usepackage{cite}
% Define superscript citation without brackets
\makeatletter
\newcommand{\supercite}[1]{%
  \begingroup
    \let\@cite\@supercite
    \cite{#1}%
  \endgroup
}

\newcommand{\@supercite}[2]{\textsuperscript{#1}}
\makeatother
\usepackage{amssymb}
\usepackage{multirow}
\usepackage{xcolor}
\usepackage{subcaption}
\usepackage{array}
\usepackage{pdflscape}
% tricks to create subsubsubsection
\usepackage{titlesec}
\usepackage{float}
\usepackage{longtable}
\setcounter{secnumdepth}{4}
\usepackage{afterpage}
\usepackage{amsmath}
\usepackage{graphicx}
\usepackage{tabularx}
\usepackage{hyperref}
\hypersetup{
    colorlinks=true,
    linkcolor=blue,
    filecolor=magenta,      
    urlcolor=cyan,
    pdftitle={Overleaf Example},
    pdfpagemode=FullScreen,
    }	
\newcommand{\indep}{\perp \!\!\! \perp}

% add line number
\usepackage{lineno}

% Page geometry.
\linespread{1.5}
\setlength{\parindent}{0cm}\geometry{
    verbose,
    tmargin=1.0in,
    bmargin=1.0in,
    lmargin=1.0in,
    rmargin=1.0in
}
\topmargin 0.0cm
\oddsidemargin 0.2cm
\textwidth 16cm 
\textheight 21cm
\footskip 1.0cm

 % New numbering for supplementary tables

\title{\bf Supplementary Materials}
\author[1]{Jianhui Gao, MS}
\author[1]{Benson Chou, BA}
\author[2]{Zachary R. McCaw, PhD}
\author[3]{Hilary Thurston, MS}
\author[4]{Paul Varghese, MD}
\author[5]{Chuan Hong, PhD}
\author[1,6,7]{Jessica Gronsbell, PhD}

\affil[1]{Department of Statistical Sciences, University of Toronto, Toronto, ON, Canada}
\affil[2]{Department of Biostatistics, Harvard T.H.\ Chan School of Public Health, Boston, MA, USA}
\affil[3]{Department of Gender \& Sexuality Studies, York University, Toronto, ON, Canada}
\affil[4]{Verily Life Sciences, Cambridge, MA, USA}
\affil[5]{Department of Biostatistics, Duke University Raleigh, NC, USA}
\affil[6]{Department of Family \& Community Medicine, University of Toronto, Toronto, ON, Canada}
\affil[7]{Department of Computer Science, University of Toronto, Toronto, ON, Canada}
\date{}

\begin{document}
\include{GrandMacros}
{
\let\newpage\relax
\maketitle
}

\tableofcontents

\newpage
\section{Comparison with Existing Literature}

\begin{table}[ht!]
\centering
\renewcommand{\arraystretch}{1.5}
\small
\centering
\begin{tabular}{|>{\centering\arraybackslash}p{0.15\textwidth}|>{\centering\arraybackslash}p{0.15\textwidth}|>{\centering\arraybackslash}p{0.15\textwidth}|>{\centering\arraybackslash}p{0.4\textwidth}|}
    \hline
    \textbf{Reference} & \textbf{Healthcare-Specific} & \textbf{Categories Covered} & \textbf{Focus on Fairness Definitions} \\
    \hline
    This Paper & \textcolor{blue}{\checkmark} & \textcolor{blue}{G, I, S, C} & \textcolor{blue}{\checkmark} \\
    \hline
    \multicolumn{4}{|l|}{\textit{Reviews and Surveys}} \\
    \hline
    \cite{ueda_fairness_2023, yfantidou_beyond_2023, chen2024unmasking} & \textcolor{blue}{\checkmark} & -- & \textcolor{red}{\texttimes} \\
    \hline
    \cite{chen_algorithmic_2023} & \textcolor{blue}{\checkmark} & G & \textcolor{red}{\texttimes} \\
    \hline
    \cite{rajkomar_ensuring_2018, wang_bias_2022, kecki_understanding_2024} & \textcolor{blue}{\checkmark} & G & \textcolor{red}{\texttimes} \\
    \hline
    \cite{anderson2024algorithmic} & \textcolor{blue}{\checkmark} & I & \textcolor{blue}{\checkmark} \\
    \hline
    \cite{makhlouf_when_2024, plecko_causal_2024} & \textcolor{red}{\texttimes} & C & \textcolor{blue}{\checkmark} \\
    \hline
    \cite{feng_fair_2022} & \textcolor{blue}{\checkmark} & G, I, C & \textcolor{blue}{\checkmark} \\
    \hline
    \cite{mitchell_prediction-based_2021, makhlouf_applicability_2021, wang_brief_2022, alves_survey_2023} & \textcolor{red}{\texttimes} & G, I, C & \textcolor{blue}{\checkmark} \\
    \hline
    \cite{mehrabi_survey_2021, pessach_review_2022, caton_fairness_2024} & \textcolor{red}{\texttimes} & G, I, S, C & \textcolor{blue}{\checkmark} \\
    \hline
    \multicolumn{4}{|l|}{\textit{Conference Workshops and Tutorials}} \\
    \hline
    \cite{bird_fairness-aware_2019} & \textcolor{red}{\texttimes} & G & \textcolor{red}{\texttimes} \\
    \hline
    \cite{ghani_addressing_2023} & \textcolor{red}{\texttimes} & G & \textcolor{red}{\texttimes} \\
    \hline
    \cite{plecko_causal_2024, nilforoshan_causal_2022} & \textcolor{red}{\texttimes} & C & \textcolor{blue}{\checkmark} \\
    \hline
    \cite{arvind_narayanan_tutorial_2018} & \textcolor{red}{\texttimes} & G, I & \textcolor{blue}{\checkmark} \\
    \hline
    \cite{farnadi_algorithmic_2022} & \textcolor{red}{\texttimes} & G, I, C & \textcolor{red}{\texttimes} \\
    \hline
    \cite{verma_fairness_2018} & \textcolor{red}{\texttimes} & G, I, C & \textcolor{blue}{\checkmark} \\
    \hline
    \cite{ahmad_fairness_2020} & \textcolor{blue}{\checkmark} & G, I, S, C & \textcolor{red}{\texttimes} \\
    \hline
\end{tabular}

\caption{\textbf{Comparison of current paper with existing literature on fairness.} G: Group fairness, I: Individual fairness, S: Subgroup fairness, C: Causality-based fairness}
\label{tab:lit-review}
\end{table}

To summarize \ref{tab:lit-review}, compared to existing literature: (i) we focus specifically on fairness definitions within healthcare applications; (ii) we demonstrate each fairness concept with real-world examples

\section{Group Fairness Criteria}
{\color{blue}
\subsection{Common Protected Attributes}
\begin{table}[ht!]
\centering
\renewcommand{\arraystretch}{1.4}
\begin{tabular}{|l|l|}
\hline
\textbf{Attribute} & \textbf{Examples} \\
\hline
Age & \cite{seyyed-kalantari_underdiagnosis_2021, garriga_machine_2022, schuch_fairness_2023, yfantidou_beyond_2023} \\
\hline
Disability & \cite{garriga_machine_2022} \\
\hline
Marital Status & \cite{wang_comparison_2022} \\
\hline
National Origin & \cite{yfantidou_beyond_2023} \\
\hline
Race & \cite{seyyed-kalantari_underdiagnosis_2021, wang_bias_2022, rajkomar_ensuring_2018, garriga_machine_2022, schuch_fairness_2023, yfantidou_beyond_2023} \\
\hline
Sex & \cite{seyyed-kalantari_underdiagnosis_2021, garriga_machine_2022, yfantidou_beyond_2023, wang_comparison_2022, yuan_algorithmic_2023} \\
\hline
Socioeconomic Status & \cite{seyyed-kalantari_underdiagnosis_2021, wang_bias_2022, rajkomar_ensuring_2018, schuch_fairness_2023, yfantidou_beyond_2023, wang_comparison_2022} \\
\hline
\end{tabular}
\caption{\textbf{Commonly used protected attributes in machine learning for health.} Examples of studies that evaluate fairness with respect to each protected attribute.}
\label{tab:protected-attributes}
\end{table}

}
\subsection{Continuous Outcomes}
While our focus in the main text is on binary outcomes, many clinical applications involve models for predicting continuous outcomes, such as healthcare costs.  The mean absolute error and mean squared error are commonly used to evaluate the performance of an algorithm when the outcome is continuous, \textcolor{black}{both of which are functions of residuals.} The parity between these metrics can also be used to evaluate fairness analogously to the setting of a binary outcome. Recently, Steinberg et al\supercite{steinberg_fairness_2020} proposed methods to measure independence, separation, and sufficiency for continuous outcomes by estimating conditional densities or using mutual information.  However, the proposed methods can only be applied in settings with binary protected attributes. \textcolor{black}{Zink and Rose\supercite{zink_fair_2020} took a different approach, exploring multiple residual-based fairness measures and incorporating them as constraints directly into the objective function in regression models. Another approach} involves conducting conditional statistical tests, such as testing independence through the Hirschfeld-Gebelein-Renyi maximal correlation coefficient, which accommodates both continuous outcomes and protected attributes.\supercite{mary_fairness-aware_2019} This is an ongoing area of research and we encourage readers to consult recent works\supercite{steinberg_fairness_2020, kim_measuring_2023} for further discussion of the topic.

\subsection{Categorical Protected Attributes}
When the protected attributes are binary, natural measures of parity include the difference or the ratio of group-specific metrics. However, many protected attributes define more than two groups, such as race and marital status.  One approach for categorical protected attributes is to directly visualize the metrics in toolkit such as AI Fairness 360.\supercite{bellamy_ai_2018} However, this method has notable limitations, including subjective judgment and challenges when dealing with numerous subgroups.\supercite{lum_-biasing_2022} To address these issues, various meta-metrics have been proposed and applied to quantify group-wise disparities into a single metric. Lum et al\supercite{lum_-biasing_2022} have summarized common meta-metrics and their limitations, which we present in Table \ref{tab:MetaMetrics} below. These metrics primarily focus on two key aspects: extremum and variability of model performances across groups.

\begin{table}[htbp!]
\centering
    \begin{tabular}{|l|l|l|}
    \hline
        \textbf{Meta-Metrics} & \textbf{Formula} & \textbf{Type} \\
        \hline 
         max-min difference & $\max_{j} \mathcal{M}_j - \min_j \mathcal{M}_j$ & Extremum \\
         \hline
         max-min ratio & $ \frac{\max_j \mathcal{M}_j}{\min_j \mathcal{M}_j}$ & Extremum \\
         \hline
         max absolute difference & $\max_j \left|\mathcal{M}_j - \frac{1}{K}\sum_{i=1}^{K}\mathcal{M}_i\right|$ & Extremum \\
         \hline
         mean absolute deviation & $\frac{1}{K} \sum_{j=1}^{K} \left|\mathcal{M}_j - \frac{1}{K}\sum_{i=1}^{K}\mathcal{M}_i\right|$ & Variability \\
         \hline
         variance & $\frac{1}{K-1} \sum_{j=1}^{K} \left(\mathcal{M}_j - \frac{1}{K}\sum_{i=1}^{K}\mathcal{M}_i\right)^2$ & Variability \\
         \hline
         generalized entropy index ($\alpha \neq 0, 1$) & $\frac{1}{K\alpha(\alpha-1)}\sum_{j=1}^{K} \left[\left(\frac{\mathcal{M}_j}{\frac{1}{K}\sum_{i=1}^{K}\mathcal{M}_i}\right)^\alpha - 1 \right]$ & Variability \\
         \hline
    \end{tabular}
    \caption{\textbf{Meta-metrics for evaluating fairness across $K$ protected groups.}  $\mathcal{M}_j$ denotes a model performance metric (e.g., the true positive rate) for $j = 1, \dots, K$. }
    \label{tab:MetaMetrics}
\end{table}

\subsection{Continuous Protected Attributes}
When dealing with continuous protected attributes, such as age, applying thresholds or bins may introduce threshold effects.\supercite{mary_fairness-aware_2019} Very recently, Mary et al\supercite{mary_fairness-aware_2019} proposed using the Hirschfeld-Gebelein-Rényi maximal correlation coefficient as a metric to measure fairness for continuous protected attributes. This is an ongoing area of research and we encourage readers to review recent works\supercite{mary_fairness-aware_2019, giuliani_generalized_2023} and references therein.

\subsection{Subgroup Fairness}
When multiple attributes are of interest (e.g., sex = \{male, female\} and race = \{white, Black\}), a model can be fair in both groups, but show disparities in an intersectional subgroup (e.g., \{Black male\}), a phenomenon known as ``Fairness Gerrymandering".\supercite{kearns_preventing_2018} Subgroup fairness or intersectional fairness selects a specific fairness constraint, such as statistical parity or equalized odds, and then evaluates it across a large collection of subgroups. For instance, a recent study evaluated a chest X-ray algorithm across the 8 possible intersectional subgroup of income = \{high, low\}, insurance = \{high, low\}, race =\{white, non-white\} by evaluating the differences between the maximum and minimum false positive rates.\supercite{moukheiber_looking_2024} 

\clearpage
\newpage

\section{Group Fairness Incompatibilities}
Formal mathematical proofs supporting these claims can be found in earlier works.\supercite{hardt_equality_2016, kleinberg2017inherent}  Below we provide a brief conceptual overview. 

\subsection{Independence versus Sufficiency}
If the outcome and protected attribute is not independent ($Y \not\indep A$), then it is not possible to achieve both independence and sufficiency. Specifically, when $Y$ is binary and prevalence differs across protected groups, an algorithm cannot simultaneously satisfy these two criteria.

\subsection{Independence versus Separation}
In addition to a lack of independence between the outcome and protected attribute ($Y \not\indep A$), if decision also depends on the outcome ($D \not\indep Y$), independence and separation are incompatible. It is important to note that this statement only holds for binary outcomes. If the prediction is not entirely uninformative for predicting the label, then there should be correlation between the prediction and the label (i.e., $D \not\indep Y$). However, with unequal prevalence across protected groups, satisfying both criteria simultaneously would yield predictions that are essentially uninformative. 

\subsection{Sufficiency versus Separation}
In addition to a lack of independence between the outcome and protected attribute ($Y \not\indep A$), if the density of the joint distribution of protected attributes, decision, and outcome $(A, D, Y)$ is strictly positive, then sufficiency and separation are incompatible. For binary outcomes, the second condition means that there is at least one false prediction. In other words, the decision cannot completely determine the outcome. Consequently, with unequal prevalences across protected groups, achieving both sufficiency and separation becomes unattainable unless the model gives perfect predictions. 

\subsection{Approximate Fairness}
A basic requirement for any of the three previously mentioned pairs to hold is that the outcome and the protected attribute are marginally independent (i.e., $Y \indep A$).  In classification problems, this means the probability of being in the positive class is the same across groups - a condition often violated in clinical contexts, where disease prevalence may vary by factors like age or sex.  While this result may be discouraging for practitioners aiming to achieve various group fairness criteria in their own applications, a relaxed notion of fairness, known as \textit{approximate fairness}\supercite{denis_fairness_2023,bell2023possibility} or $\epsilon$-fairness, allows for a small margin of error in the group fairness metrics presented in Table 3 in the main text. That is, rather than enforcing exact equality of metrics across groups, approximate fairness deems a model fair if the difference between metrics does not exceed some small value, $\epsilon$.\supercite{bell2023possibility} demonstrates that it is possible for an model to satisfy approximate fairness across the false negative rate, false positive rate, and positive predictive value, even when moderate prevalence differences between groups exist. This finding is promising for health-focused applications where exact parity is often unachievable.

\clearpage

\begin{singlespace}
\bibliographystyle{wileyNJD-AMA}
\bibliography{references}
\end{singlespace}

\end{document}
