# Supplementary material for: What is Fair? Defining Fairness in Machine Learning for Health
Source: arXiv:2406.09307 source file (2025-05-27)
Supplement: Supplementary file 4 [file supplementary.tex]

\documentclass[12pt]{article}

% Package
\usepackage{geometry}
\usepackage[utf8]{inputenc}
\usepackage{authblk}
\renewcommand\Affilfont{\fontsize{11}{11}\itshape}
\usepackage{setspace}
\usepackage[backend=biber,style=nature, isbn=false,url=false,eprint=false]{biblatex}
\addbibresource{references.bib}
\usepackage{amssymb}
\usepackage{multirow}
\usepackage{xcolor}
\usepackage{subcaption}
\usepackage{array}
\usepackage{pdflscape}
% tricks to create subsubsubsection
\usepackage{titlesec}
\usepackage{float}
\usepackage{longtable}
\setcounter{secnumdepth}{4}
\usepackage{afterpage}
\usepackage{amsmath}
\usepackage{graphicx}
\usepackage{tabularx}
\usepackage{hyperref}
\hypersetup{
    colorlinks=true,
    linkcolor=blue,
    filecolor=magenta,      
    urlcolor=cyan,
    pdftitle={Overleaf Example},
    pdfpagemode=FullScreen,
    }	
\newcommand{\indep}{\perp \!\!\! \perp}

% add line number
\usepackage{lineno}


% Page geometry.
\linespread{1.5}
\setlength{\parindent}{0cm}\geometry{
    verbose,
    tmargin=1.0in,
    bmargin=1.0in,
    lmargin=1.0in,
    rmargin=1.0in
}
\topmargin 0.0cm
\oddsidemargin 0.2cm
\textwidth 16cm 
\textheight 21cm
\footskip 1.0cm

\renewcommand{\thetable}{S\arabic{table}} % New numbering for supplementary tables

\title{\bf Supplementary Materials}
\author[1]{Jianhui Gao, MS}
\author[1]{Benson Chou, BA}
\author[2]{Zachary R. McCaw, PhD}
\author[3]{Hilary Thurston, MS}
\author[4]{Paul Varghese, MD}
\author[5]{Chuan Hong, PhD}
\author[1,6,7]{Jessica Gronsbell, PhD}

\affil[1]{Department of Statistical Sciences, University of Toronto, Toronto, ON, Canada}
\affil[2]{Department of Biostatistics, Harvard T.H.\ Chan School of Public Health, Boston, MA, USA}
\affil[3]{Department of Gender \& Sexuality Studies, York University, Toronto, ON, Canada}
\affil[4]{Verily Life Sciences, Cambridge, MA, USA}
\affil[5]{Department of Biostatistics, Duke University Raleigh, NC, USA}
\affil[6]{Department of Family \& Community Medicine, University of Toronto, Toronto, ON, Canada}
\affil[7]{Department of Computer Science, University of Toronto, Toronto, ON, Canada}
\date{}

\begin{document}
\include{GrandMacros}
{
\let\newpage\relax
\maketitle
}


\tableofcontents


\newpage
\section{Comparison with Existing Literature}
\begin{table}[ht!]
\centering
\renewcommand{\arraystretch}{1.5}

\tiny
\centering
\begin{tabular}{|>{\centering\arraybackslash}p{0.1\textwidth}|>{\centering\arraybackslash}p{0.09\textwidth}|>{\centering\arraybackslash}p{0.08\textwidth}|>{\centering\arraybackslash}p{0.14\textwidth}|>{\centering\arraybackslash}p{0.14\textwidth}|>{\centering\arraybackslash}p{0.1\textwidth}|>{\centering\arraybackslash}p{0.15\textwidth}|}
    \hline
       \multirow{2}{*}{\textbf{Reference}} & \textbf{Healthcare-Specific} & \textbf{Categories Covered} & \textbf{Focus on Fairness Definitions} & \textbf{Illustrated with  Real-world Data}  & \textbf{Reproducible Code} & \textbf{Format}  \\ 
       \hline
       This Paper  & \textcolor{blue}{\checkmark} & \textcolor{blue}{G, I, S, C} & \textcolor{blue}{\checkmark} & \textcolor{blue}{\checkmark} & \textcolor{blue}{\texttt{R}} & Article \\
       \hline
       \multicolumn{7}{|l|}{\textit{Reviews and Surveys}} \\
       \hline
       \cite{ueda_fairness_2023, yfantidou_accuracy_2023, chen2024unmasking} & \textcolor{blue}{\checkmark} & -- & \textcolor{red}{\texttimes}&\textcolor{red}{\texttimes} & \textcolor{red}{\texttimes} & Article\\
       \hline
    \cite{chen_algorithmic_2023} & \textcolor{blue}{\checkmark} & G & \textcolor{red}{\texttimes}& \textcolor{red}{\texttimes} & \textcolor{red}{\texttimes} & Article\\
       \hline
       \cite{rajkomar_ensuring_2018, wang_bias_2022, kecki_understanding_2024} & \textcolor{blue}{\checkmark} & G & \textcolor{red}{\texttimes}&\textcolor{blue}{\checkmark} & \textcolor{red}{\texttimes} & Article \\
       \hline
       \cite{anderson2024algorithmic} &  \textcolor{blue}{\checkmark} & I &  \textcolor{blue}{\checkmark} & \textcolor{red}{\texttimes} & \textcolor{red}{\texttimes} & Article\\
       \hline
       \cite{makhlouf_when_2024, plecko_causal_2024} & \textcolor{red}{\texttimes} & C &  \textcolor{blue}{\checkmark} &  \textcolor{red}{\texttimes} & \textcolor{red}{\texttimes} & Article\\
       \hline
       \cite{feng_fair_2022} & \textcolor{blue}{\checkmark} & G, I, C & \textcolor{blue}{\checkmark} & \textcolor{red}{\texttimes} & \textcolor{red}{\texttimes} & Article \\
       \hline
       \cite{mitchell_prediction-based_2021, makhlouf_applicability_2021, wang_brief_2022, alves_survey_2023} & \textcolor{red}{\texttimes} & G, I, C & \textcolor{blue}{\checkmark} & \textcolor{red}{\texttimes} & \textcolor{red}{\texttimes} & Article \\ 
       \hline
       \cite{mehrabi_survey_2021, pessach_review_2022, caton_fairness_2024} & \textcolor{red}{\texttimes} & G, I, S, C & \textcolor{blue}{\checkmark}  & \textcolor{red}{\texttimes} & \textcolor{red}{\texttimes} & Article\\
       \hline
       \multicolumn{7}{|l|}{\textit{Conference Workshops and Tutorials}}\\
       \hline
        \cite{bird_fairness-aware_2019} & \textcolor{red}{\texttimes}& G  & \textcolor{red}{\texttimes} &\textcolor{blue}{\checkmark} &\textcolor{red}{\texttimes} & Slides, Video \\
        \hline
       \cite{ghani_addressing_2023} & \textcolor{red}{\texttimes} & G & \textcolor{red}{\texttimes}  & \textcolor{blue}{\checkmark} & \textcolor{blue}{\texttt{Python}} & Slides, Video \\
       \hline
       \cite{plecko_causal_2022, nilforoshan_causal_2022} & \textcolor{red}{\texttimes} & C &\textcolor{blue}{\checkmark} & \textcolor{red}{\texttimes} & \textcolor{red}{\texttimes} & Article, Slides, Video \\
       \hline
\cite{arvind_narayanan_tutorial_2018} & \textcolor{red}{\texttimes} & G, I &\textcolor{blue}{\checkmark} & \textcolor{red}{\texttimes} & \textcolor{red}{\texttimes} & Video \\
       \hline
       \cite{farnadi_algorithmic_2022} & \textcolor{red}{\texttimes} & G, I, C & \textcolor{red}{\texttimes} & \textcolor{red}{\texttimes}  & \textcolor{red}{\texttimes} & Slides, Video\\
       \hline
       \cite{verma_fairness_2018} & \textcolor{red}{\texttimes} & G, I, C & \textcolor{blue}{\checkmark}  & \textcolor{blue}{\checkmark} &  \textcolor{red}{\texttimes} & Article, Slides\\
       \hline
        \cite{ahmad_fairness_2020} & \textcolor{blue}{\checkmark} & G, I, S, C & \textcolor{red}{\texttimes} & \textcolor{blue}{\checkmark} & \textcolor{blue}{\texttt{Python}} & Slides\\
       \hline
       \end{tabular}

\caption{\textbf{Comparison of current paper with existing literature on fairness.} G: Group  fairness, I: Individual fairness, S: Subgroup fairness, C: Causality-based fairness}
\label{tab:lit-review}
\end{table}

To summarize \ref{tab:lit-review}, compared to existing literature: (i) we focus specifically on fairness definitions within healthcare applications; (ii) we demonstrate each fairness concept with real-world examples; (iii) we provide a fully reproducible case study of mortality prediction on publicly available EHR data from the Medical Information Mart for Intensive Care (MIMIC) clinical database \cite{raffa2016clinical}.

\section{Group Fairness Criteria}
\subsection{Continuous Outcome}
While our focus in the main text is on binary outcomes, many clinical applications involve models for predicting continuous outcomes, such as healthcare costs.  The mean absolute error and mean squared error are commonly used to evaluate the performance of an algorithm when the outcome is continuous, \textcolor{blue}{both of which are functions of residuals.} The parity between these metrics can also be used to evaluate fairness analogously to the setting of a binary outcome. Recently, \cite{steinberg_fairness_2020} proposed methods to measure independence, separation, and sufficiency for continuous outcomes by estimating conditional densities or using mutual information.  However, the proposed methods can only be applied in settings with binary protected attributes. \textcolor{blue}{Zink and Rose \cite{zink_fair_2020} took a different approach, exploring multiple residual-based fairness measures and incorporating them as constraints directly into the objective function in regression models. Another approach} involves conducting conditional statistical tests, such as testing independence through the Hirschfeld-Gebelein-Renyi maximal correlation coefficient, which accommodates both continuous outcomes and protected attributes \cite{mary_fairness-aware_2019}. This is an ongoing area of research and we encourage readers to consult \cite{steinberg_fairness_2020, kim_measuring_2023} for further discussion of the topic.

\subsection{Categorical Protected Attributes}
When the protected attributes are binary, natural measures of parity include the difference or the ratio of group-specific metrics. However, many protected attributes define more than two groups, such as race and marital status.  One approach for categorical protected attributes is to directly visualize the metrics in toolkit such as AI Fairness 360 \cite{bellamy_ai_2018}. However, this method has notable limitations, including subjective judgment and challenges when dealing with numerous subgroups \cite{lum_-biasing_2022}. To address these issues, various meta-metrics have been proposed and applied to quantify group-wise disparities into a single metric. \cite{lum_-biasing_2022} have summarized common meta-metrics and their limitations, which we present in Table \ref{tab:MetaMetrics} below. These metrics primarily focus on two key aspects: extremum and variability of model performances across groups. 


\begin{table}[htbp!]
\centering
    \begin{tabular}{|l|l|l|}
    \hline
        \textbf{Meta-Metrics} & \textbf{Formula} & \textbf{Type} \\
        \hline 
         max-min difference & $\max_{j} \mathcal{M}_j - \min_j \mathcal{M}_j$ & Extremum \\
         \hline
         max-min ratio & $ \frac{\max_j \mathcal{M}_j}{\min_j \mathcal{M}_j}$ & Extremum \\
         \hline
         max absolute difference & $\max_j \left|\mathcal{M}_j - \frac{1}{K}\sum_{i=1}^{K}\mathcal{M}_i\right|$ & Extremum \\
         \hline
         mean absolute deviation & $\frac{1}{K} \sum_{j=1}^{K} \left|\mathcal{M}_j - \frac{1}{K}\sum_{i=1}^{K}\mathcal{M}_i\right|$ & Variability \\
         \hline
         variance & $\frac{1}{K-1} \sum_{j=1}^{K} \left(\mathcal{M}_j - \frac{1}{K}\sum_{i=1}^{K}\mathcal{M}_i\right)^2$ & Variability \\
         \hline
         generalized entropy index ($\alpha \neq 0, 1$) & $\frac{1}{K\alpha(\alpha-1)}\sum_{j=1}^{K} \left[\left(\frac{\mathcal{M}_j}{\frac{1}{K}\sum_{i=1}^{K}\mathcal{M}_i}\right)^\alpha - 1 \right]$ & Variability \\
         \hline
    \end{tabular}
    \caption{\textbf{Meta-metrics for evaluating fairness across $K$ protected groups.}  $\mathcal{M}_j$ denotes a model performance metric (e.g., the true positive rate) for $j = 1, \dots, K$. }
    \label{tab:MetaMetrics}
\end{table}

\subsection{Continuous Protected Attributes}
When dealing with continuous protected attributes, such as age, applying thresholds or bins may introduce threshold effects \cite{mary_fairness-aware_2019}. Very recently, \cite{mary_fairness-aware_2019} proposed using the Hirschfeld-Gebelein-Rényi maximal correlation coefficient as a metric to measure fairness for continuous protected attributes. This is an ongoing area of research and we encourage readers to review \cite{mary_fairness-aware_2019, giuliani_generalized_2023} and references therein.


\subsection{Subgroup Fairness}
When multiple attributes are of interest (e.g., sex = \{male, female\} and race = \{white, Black\}), a model can be fair in both groups, but show disparities in an intersectional subgroup (e.g., \{Black male\}), a phenomenon known as ``Fairness Gerrymandering" \cite{kearns_preventing_2018}. Subgroup fairness or intersectional fairness selects a specific fairness constraint, such as statistical parity or equalized odds, and then evaluates it across a large collection of subgroups. For instance, a recent study evaluated a chest X-ray algorithm across the 8 possible intersectional subgroup of income = \{high, low\}, insurance = \{high, low\}, race =\{white, non-white\} by evaluating the differences between the maximum and minimum false positive rates \cite{moukheiber_looking_2024}. 

\clearpage
\newpage

\section{Group Fairness Incompatibilities}
Formal mathematical proofs supporting these claims can be found in \cite{hardt_equality_2016, kleinberg2017inherent}.  Below we provide a brief conceptual overview. 

\subsection{Independence versus Sufficiency}
If the outcome and protected attribute is not independent ($Y \not\indep A$), then it is not possible to achieve both independence and sufficiency. Specifically, when $Y$ is binary and prevalence differs across protected groups, an algorithm cannot simultaneously satisfy these two criteria.

\subsection{Independence versus Separation}
In addition to a lack of independence between the outcome and protected attribute ($Y \not\indep A$), if decision also depends on the outcome ($D \not\indep Y$), independence and separation are incompatible. It is important to note that this statement only holds for binary outcomes. If the prediction is not entirely uninformative for predicting the label, then there should be correlation between the prediction and the label (i.e., $D \not\indep Y$). However, with unequal prevalence across protected groups, satisfying both criteria simultaneously would yield predictions that are essentially uninformative. 

\subsection{Sufficiency versus Separation}
In addition to a lack of independence between the outcome and protected attribute ($Y \not\indep A$), if the density of the joint distribution of protected attributes, decision, and outcome $(A, D, Y)$ is strictly positive, then sufficiency and separation are incompatible. For binary outcomes, the second condition means that there is at least one false prediction. In other words, the decision cannot completely determine the outcome. Consequently, with unequal prevalences across protected groups, achieving both sufficiency and separation becomes unattainable unless the model gives perfect predictions. 

\subsection{Approximate Fairness}
A basic requirement for any of the three previously mentioned pairs to hold is that the outcome and the protected attribute are marginally independent (i.e., $Y \indep A$).  In classification problems, this means the probability of being in the positive class is the same across groups - a condition often violated in clinical contexts, where disease prevalence may vary by factors like age or sex.  While this result may be discouraging for practitioners aiming to achieve various group fairness criteria in their own applications, a relaxed notion of fairness, known as \textit{approximate fairness} or $\epsilon$-fairness, allows for a small margin of error in the group fairness metrics presented in Table 3 in the main text \cite{denis_fairness_2023,bell2023possibility}. That is, rather than enforcing exact equality of metrics across groups, approximate fairness deems a model fair if the difference between metrics does not exceed some small value, $\epsilon$. \cite{bell2023possibility} demonstrates that it is possible for an model to satisfy approximate fairness across the false negative rate, false positive rate, and positive predictive value, even when moderate prevalence differences between groups exist. This finding is promising for health-focused applications where exact parity is often unachievable. 

\newpage

\section{Case Study}

To illustrate the incompatibilities between different fairness notions, we consider a case study using a publicly available dataset on 1,776 ICU patients from MIMIC-II \cite{mitcriticaldata2016secondary, raffa2016clinical}\footnote{While MIMIC-IV is the latest version of the database, access is restricted to credentialed users through PhysioNet \cite{goldberger_physiobank_2000}. The dataset used in this case study, however, is publicly available to everyone, making it easy to replicate}, focusing on predicting 28-day mortality and evaluating disparities in model performance across sex \footnote{We acknowledge that sex is not binary, but recorded as either male or female in the MIMIC-II data \cite{lancaster2023complexities}.}.  We describe the model building procedures and results in the subsequent subsections while the details of the methods used to obtain the 95\% confidence intervals (CIs) are provided in Supplementary Section 5. 

\subsection{Dataset}
The dataset has been used to investigate the relationship between indwelling arterial catheters in hemodynamically stable patients and respiratory failure regarding mortality outcomes \cite{raffa2016clinical}.  It includes 46 variables, including demographics, clinical characteristics such as white blood cell count and heart rate during ICU stays, and a 28-day mortality indicator on 1,776 patients. The data is publicly available at \url{https://physionet.org/content/mimic2-iaccd/1.0/}.

\subsection{Data Preprocessing}
We removed three variables that had more than 10\% missing values: body mass index (26.2\%), first partial pressure of oxygen (10.5\%), and first partial pressure of carbon dioxide (10.5\%). For the remaining variables with missing values, we imputed the missing data with their respective medians. Additionally, we removed the variable `sepsis\_flg' as it was absent in all records. Lastly, four variables - death in hospital, death in ICU, day post ICU admission of censoring or death, and censored or death - were removed because they cannot be used as predictors for mortality as they are dependent on the outcome being predicted. All analyses utilized an R package that we developed and can be replicated using the code at: \url{https://jianhuig.github.io/FairnessTutorial/index.html}

\subsection{Model Building}
We used the first 700 observations as the training set to fit a random forest (RF) model and the remaining 1,076 observations as the testing set. The hyperparameters for the RF model were set to use 1000 trees and a random sampling of 6 variables at each split, determined by the square root of the number of predictors. The overall area under the receiver operating characteristic curve (AUC) for our model on the test set is 0.90. Additionally, the overall accuracy of the model on the test set is 0.88. We selected a cut-off value of 0.41 for fairness evaluation, as it achieves a false positive rate (FPR) of approximately 5\%.

\subsection{Results}
The results from the analyses are presented in Table \ref{tab:real-data}.\\

Independence is likely violated, as evidenced by the statistical parity metric showing a 9\% difference (95\% CI: [5\%, 13\%]) or a ratio of 2.12 (95\% CI: [1.49, 3.04]) between females and males. The measures in the independence category indicate that the model predicts a significantly higher mortality rate for females, even after conditioning on age. \\

With respect to separation, we observe that all metrics show significant disparities. For instance, equal opportunity shows a -24\% difference (95\% CI: [-39\%, -9\%]) in false negative rate (FNR) between females and males. This indicates our model is less likely to detect males at risk of mortality compared to females. \\

On the other hand, the sufficiency criterion is satisfied as predictive parity shows no significant difference between males and females (difference: -4\%, 95\% CI: [-21\%, 13\%]; ratio: 0.94, 95\% CI: [0.72, 1.23]). This suggests that given the same prediction, the actual mortality rates are similar for both males and females. \\

Lastly, three additional metrics from Table \ref{tab:real-data} that do not fall within the three aforementioned categories that measure calibration and/or discrimination are satisfied.

\subsection{Practical Considerations}

In our case study, both separation and sufficiency-based metrics are important. Separation ensures that patients at a true risk of mortality are accurately identified across protected groups. This reduces the risk of systematically under-detecting individuals who may require immediate intervention in a particular subpopulation. On the other hand, sufficiency is also valuable, as it ensures that immediate intervention is based sorely on predicted medical needs rather than other protected attributes. \\

However, 28-day-mortality is unlikely to be marginally independent of sex as the estimated mortality rates differ between females (19\%) and males (14\%). As a consequence, it is not possible for the model to simultaneously satisfy more than one fairness category due to the previously discussed incompatibilities. This points to the complexity of fairness considerations in clinical settings, where one must prioritize which criteria are most relevant. Given the different mortality rates between males and females, enforcing independence is likely not advisable, as it could blind the model to true mortality rate differences. Our model violates separation criteria, which could result in higher rates of undetected mortality risk among male patients and potential delays in interventions to their care. In the main text, we reference several resources for bias mitigation strategies that can potentially help reduce the observed disparities in separation-based metrics.

\begin{table}[ht]
\resizebox{\textwidth}{!}{%
    \begin{tabular}{|l|c|c|c|c|c|c|}
    \hline
    \textbf{Fairness Metric} & \textbf{Female} & \textbf{Male} & \textbf{Difference} & \textbf{95\% CI for the difference} & \textbf{Ratio} & \textbf{95\% CI for the ratio}\\ \hline
    \multicolumn{7}{|l|}{\textit{Independence-based criteria}} \\ \hline
    Statistical Parity  & 17\% & 8\% & 9\% & [5\%, 13\%] & 2.12 & [1.49, 3.04]\\ \hline
    Conditional Statistical Parity (Age $\geq 60$) & 34\% & 21\% & 13\% & [5\%, 21\%] & 1.62 & [1.17, 2.23]\\ \hline
    \multicolumn{7}{|l|}{\textit{Separation-based criteria}} \\ \hline
    Equal Opportunity  & 38\% & 62\% & -24\% & [-39\%, -9\%] & 0.61 & [0.44, 0.86]\\ \hline
    Predictive Equality  & 8\% & 3\% & 5\% & [2\%, 8\%] & 2.67 & [1.39, 5.12]\\ \hline
    Balance for Positive Class & 46\% & 37\% & 9\% & [4\%, 14\%] & 1.24 & [1.09, 1.42]\\ \hline
    Balance for Negative Class & 15\% & 10\% & 5\% & [3\%, 7\%] & 1.5 & [1.28, 1.75]\\ \hline
    \multicolumn{7}{|l|}{\textit{Sufficiency-based criteria}} \\ \hline
    Predictive Parity  & 62\% & 66\% & -4\% & [-21\%, 13\%] & 0.94 & [0.72, 1.23]\\ \hline
    \multicolumn{7}{|l|}{\textit{Other criteria}} \\ \hline
    Brier Score Parity & 9\% & 8\% & 1\% & [-1\%, 3\%] & 1.12 & [0.89, 1.42]\\ \hline
    Overall Accuracy Equality & 87\% & 88\% & -1\% & [-5\%, 3\%] & 0.99 & [0.94, 1.04]\\ \hline
    Treatment Equality & 5.11 & 13.6 & -8.49 & [-32.96, 15.98] & 0.38 & [0.1, 1.34]\\ \hline
    \end{tabular}}
    \caption{\textbf{Group fairness evaluation in the MIMIC-II mortality case study.}    Each metric quantifies disparities in model performance across males and females. Differences and ratios are presented alongside 95\% confidence intervals (CIs).}
    \label{tab:real-data}
\end{table}

\clearpage

\section{Construction of Confidence Intervals}
We illustrate the procedure for constructing confidence intervals (CIs) using the false positive rate (FPR) as an example. Let $\widehat{\textrm{FPR}}_a$ and $\textrm{FPR}_a$ represent the estimated and true FPRs in group $a \in \mathcal{A}$. We construct Wald-type CIs using the following result: $\sqrt{n} \left(\widehat{\textrm{FPR}}_a - \textrm{FPR}_a \right)$ is asymptotic normal with mean 0 for all $a \in \mathcal{A}$ \cite[e.g.,][]{gronsbell2018semisupervised,    gao2024semisupervised}. Let $\widehat{\Delta}_{\textrm{FPR}} = \widehat{\textrm{FPR}}_{a_1} - \widehat{\textrm{FPR}}_{a_0}$ represent the estimated difference between group $a_1$ and $a_0$. It follows that $\sqrt{n}\left(\widehat{\Delta}_{\textrm{FPR}} - \Delta_{\textrm{FPR}}\right)$ is asymptotic normal with mean 0. To estimate the standard error of $\widehat{\Delta}_{\textrm{FPR}}$, we utilize the non-parametric bootstrap \cite{efron1986bootstrap}. For each bootstrap iteration $b$ in \{1,..., B\}, we sample the data with replacement within each group and then calculate $\widehat{\Delta}_{\textrm{FPR}}^{(b)}$. Note that resampling within groups assumes that the group sizes are fixed.  The estimated standard error is the empirical standard error of the difference:
\begin{equation*}
    \widehat{\textrm{se}}\left[\widehat{\Delta}_{\textrm{FPR}}\right] = \sqrt{\frac{1}{B-1}\sum_{b=1}^B \left(\widehat{\Delta}_{\textrm{FPR}}^{(b)} - \frac{1}{B} \sum_{b=1}^B \widehat{\Delta}_{\textrm{FPR}}^{(b)}\right)^2}.
\end{equation*}
The corresponding Wald-based $100(1-\alpha)\%$ CI is given by $\widehat{\Delta}_{\textrm{FPR}} \pm z_{1-\alpha/2} * \widehat{\textrm{se}}\left[\widehat{\Delta}_{\textrm{FPR}}\right] $, where $z_{1-\alpha/2}$ is the $100(1-\alpha/2)$ percentile of the standard normal distribution. \\

To construct a $100(1-\alpha)\%$ Wald-type CI for the ratio $\widehat{\rho}_{\textrm{FPR}} = \frac{\widehat{\textrm{FPR}}_{a_1}}{\widehat{\textrm{FPR}}_{a_0}}$, we note that $\sqrt{n}\left[\log\left(\widehat{\rho}_{\textrm{FPR}}\right)- \log\left(\rho_{\textrm{FPR}}\right)\right]$ is asymptotic normal with mean 0. For each bootstrap iteration $b$ in \{1,..., B\}, we sample the data with replacement within each group and then calculate $\log\left[\widehat{\rho}_{\textrm{FPR}}^{(b)}\right]$. The estimated standard error of the log ratio is:
\begin{equation*}
\widehat{\textrm{se}}\left[\log\left(\widehat{\rho}_{\textrm{FPR}}\right)\right] = \sqrt{\frac{1}{B-1}\sum_{b=1}^B \left\{\log\left[\widehat{\rho}_{\textrm{FPR}}^{(b)}\right] - \frac{1}{B} \sum_{b=1}^B \log\left[\widehat{\rho}_{\textrm{FPR}}^{(b)}\right]\right\}^2}.
\end{equation*}
The corresponding $100(1-\alpha)\%$ CI is given by $\exp \left\{\log\left[\widehat{\rho}_{\textrm{FPR}}\right] \pm z_{1-\alpha/2} * \widehat{\textrm{se}}\left[\log\left(\widehat{\rho}_{\textrm{FPR}}\right)\right]\right\} $, where $z_{1-\alpha/2}$ is the $100(1-\alpha/2)$ percentile of the standard normal distribution. 

\clearpage
\nolinenumbers
\begin{singlespace}
\printbibliography
\end{singlespace}

\end{document}

https://arxiv.org/pdf/1909.00066

https://www.sciencedirect.com/science/article/pii/S2193943823000067

Counterfactual fairness & $P(D = 1 \mid \bZ) = P(D(a') = 1) \mid \bZ$, where $D(a')$ denotes when one's protected attribute is counterfactually altered to $a'\in \Asc$\\

\section*{Supplementary Information for Categorical Attributes}
To illustrate auditing fairness when the protected attributes are categorical, we used data from PheCAP package, which used natural language processing (NLP) to extract structured data and information from electronic medical record narrative notes. We categorized the data into four groups based on the healthcare utilization variable and fit a logistic regression model on the outcome and NLP extracted variables. We then input the predictions and outcomes into our FairnessTutorial package to evaluate the multi-group meta metrics as shown in Table \ref{tab:MultiGroupVer2}.

\begin{table}[ht]
\resizebox{\textwidth}{!}{  
        \centering
        \begin{tabular}{|l|l|l|l|l|l|l|l|l|l|l|}
             \hline
             \textbf{Metric} & \textbf{Group 1} & \textbf{Group 2} & \textbf{Group 3} & \textbf{Group 4} & Max-Min & Max/Min  & Max Abs Diff & Mean Abs Dev & Variance & Generalized Entropy Index \\ \hline
            TPR & 0.37 & 0.65 & 0.73 & 0.73 & 0.36 & 1.97 & 0.11 & 0.16,  & 0.03 & 0.03\\ \hline
            FPR & 0.02 & 0.13 & 0.09 & 0.20 & 0.18 & 10.00 & 0.9 & 0.08 & 0.01 & 0.18 \\
            \hline
            PPR & 0.16 & 0.27 & 0.34 & 0.49 & 0.33 & 3.06 & 0.17 & 0.15 & 0.02 & 0.07 \\
            \hline
            PPV & 0.94 & 0.83 & 0.89 & 0.79 & 0.15 & 1.19 & 0.08 & 0.08 & 0.00 & 0.00 \\
            \hline
            NPV & 0.69 & 0.83 & 0.83 & 0.71 & 0.14 & 1.20 & 0.07 & 0.10 & 0.01 & 0.00 \\
            \hline
            ACC & 0.73 & 0.83 & 0.85 & 0.75 & 0.12 & 1.16 & 0.06 & 0.07 & 0.00 & 0.00 \\
            \hline
            Brier Score & 0.17 & 0.12 & 0.11 & 0.17 & 0.06 & 1.55 & 0.03 & 0.04 & 0.01 & 0.02 \\
            \hline
            FN/FP Ratio & 27.67 & 2.69 & 3.04 & 1.37 & 26.3 & 20.20 & 18.98 & 9.88 & 160.58 & 0.80 \\
            \hline
            Avg Pred Prob & 0.37 & 0.37 & 0.41 & 0.52 & 0.15 & 1.41 & 0.10 & 0.07 & 0.01 & 0.01 \\
            \hline
        \end{tabular}}
        \caption{\textbf{Results for the PheCAP example.}}
        \label{tab:MultiGroupVer2}
    \end{table}

\iffalse
\begin{table}[ht]
    \centering
    \caption{MultiGroup Meta-Metrics} \label{tab:MultiGroup}
    \begin{subtable}{\textwidth}
    \centering
    \caption{Max Min Difference}
    \begin{tabular}{|l|l|l|l|l|l|l|}
    \hline
    Metric & Group 1 & Group 2 & Group 3 & Group 4 & Max-Min & 95\% CI \\ \hline
    TPR & 0.37 & 0.65 & 0.73 & 0.73 & 1.97 & [5.33,5.33] \\ \hline
    FPR & 0.02 & 0.13 & 0.09 & 0.20 & 10.00 & [500,500] \\ \hline
    PPR & 0.16 & 0.27 & 0.34 & 0.49 & 3.06 & [19.14,19.14] \\ \hline
    PPV & 0.94 & 0.83 & 0.89 & 0.79 & 1.19 & [1.51,1.51] \\ \hline
    NPV & 0.69 & 0.83 & 0.83 & 0.71 & 1.20 & [1.74,1.74] \\ \hline
    ACC & 0.73 & 0.83 & 0.85 & 0.75 & 1.16 & [1.6,1.6] \\ \hline
    Brier Score & 0.17 & 0.12 & 0.11 & 0.17 & 1.55 & [14.05,14.05] \\ \hline
    FN/FP Ratio & 27.67 & 2.69 & 3.04 & 1.37 & 20.20 & [20.2,20.2] \\ \hline
    Avg Pred Prob & 0.37 & 0.37 & 0.41 & 0.52 & 1.41 & [3.8,3.8] \\ \hline
    \end{tabular}
    \end{subtable}

    \begin{subtable}{\textwidth}
    \centering
    \caption{Max Min Ratio}
    \begin{tabular}{|l|l|l|l|l|l|l|}
    \hline
    Metric & Group 1 & Group 2 & Group 3 & Group 4 & Max/Min & 95\% CI \\ \hline
    TPR & 0.37 & 0.65 & 0.73 & 0.73 & 1.97 & [5.33,5.33] \\ \hline
    FPR & 0.02 & 0.13 & 0.09 & 0.20 & 10.00 & [500,500] \\ \hline
    PPR & 0.16 & 0.27 & 0.34 & 0.49 & 3.06 & [19.14,19.14] \\ \hline
    PPV & 0.94 & 0.83 & 0.89 & 0.79 & 1.19 & [1.51,1.51] \\ \hline
    NPV & 0.69 & 0.83 & 0.83 & 0.71 & 1.20 & [1.74,1.74] \\ \hline
    ACC & 0.73 & 0.83 & 0.85 & 0.75 & 1.16 & [1.6,1.6] \\ \hline
    Brier Score & 0.17 & 0.12 & 0.11 & 0.17 & 1.55 & [14.05,14.05] \\ \hline
    FN/FP Ratio & 27.67 & 2.69 & 3.04 & 1.37 & 20.20 & [20.2,20.2] \\ \hline
    Avg Pred Prob & 0.37 & 0.37 & 0.41 & 0.52 & 1.41 & [3.8,3.8] \\ \hline
    \end{tabular}
    \end{subtable}

    \begin{subtable}{\textwidth}
    \centering
    \caption{Max Absolute Difference}
    \begin{tabular}{|l|l|l|l|l|l|l|}
    \hline
    Metric & Group 1 & Group 2 & Group 3 & Group 4 & Max\_Abs\_Diff & 95\% CI \\ \hline
    TPR & 0.37 & 0.65 & 0.73 & 0.73 & 0.11 & [0.21,0.21] \\ \hline
    FPR & 0.02 & 0.13 & 0.09 & 0.20 & 0.09 & [0.09,0.09] \\ \hline
    PPR & 0.16 & 0.27 & 0.34 & 0.49 & 0.17 & [0.2,0.2] \\ \hline
    PPV & 0.94 & 0.83 & 0.89 & 0.79 & 0.08 & [0.23,0.23] \\ \hline
    NPV & 0.69 & 0.83 & 0.83 & 0.71 & 0.07 & [0.2,0.2] \\ \hline
    ACC & 0.73 & 0.83 & 0.85 & 0.75 & 0.06 & [0.21,0.21] \\ \hline
    Brier Score & 0.17 & 0.12 & 0.11 & 0.17 & 0.03 & [0.05,0.05] \\ \hline
    FN/FP Ratio & 27.67 & 2.69 & 3.04 & 1.37 & 18.98 & [16.92,16.92] \\ \hline
    Avg Pred Prob & 0.37 & 0.37 & 0.41 & 0.52 & 0.10 & [0.17,0.17] \\ \hline
    \end{tabular}
    \end{subtable}
    
    \begin{subtable}{\textwidth}
    \centering
    \caption{Mean Absolute Deviation}
    \begin{tabular}{|l|l|l|l|l|l|l|}
    \hline
    Metric & Group 1 & Group 2 & Group 3 & Group 4 & Mean\_Abs\_Dev & 95\% CI \\ \hline
    TPR & 0.37 & 0.65 & 0.73 & 0.73 & 0.16 & [0.12,0.21] \\ \hline
    FPR & 0.02 & 0.13 & 0.09 & 0.20 & 0.08 & [0.05,0.11] \\ \hline
    PPR & 0.16 & 0.27 & 0.34 & 0.49 & 0.15 & [0.12,0.17] \\ \hline
    PPV & 0.94 & 0.83 & 0.89 & 0.79 & 0.08 & [0.04,0.11] \\ \hline
    NPV & 0.69 & 0.83 & 0.83 & 0.71 & 0.10 & [0.06,0.13] \\ \hline
    ACC & 0.73 & 0.83 & 0.85 & 0.75 & 0.07 & [0.05,0.1] \\ \hline
    Brier Score & 0.17 & 0.12 & 0.11 & 0.17 & 0.04 & [0.03,0.06] \\ \hline
    FN/FP Ratio & 27.67 & 2.69 & 3.04 & 1.37 & 9.88 & [5.15,33.36] \\ \hline
    Avg Pred Prob & 0.37 & 0.37 & 0.41 & 0.52 & 0.07 & [0.05,0.09] \\ \hline
    \end{tabular}
    \end{subtable}
    
    \begin{subtable}{\textwidth}
    \centering
    \caption{Variance}
    \begin{tabular}{|l|l|l|l|l|l|l|}
    \hline
    Metric & Group 1 & Group 2 & Group 3 & Group 4 & Variance & 95\% CI \\ \hline
    TPR & 0.37 & 0.65 & 0.73 & 0.73 & 0.03 & [0.02,0.04] \\ \hline
    FPR & 0.02 & 0.13 & 0.09 & 0.20 & 0.01 & [0,0.01] \\ \hline
    PPR & 0.16 & 0.27 & 0.34 & 0.49 & 0.02 & [0.01,0.03] \\ \hline
    PPV & 0.94 & 0.83 & 0.89 & 0.79 & 0.00 & [0,0.01] \\ \hline
    NPV & 0.69 & 0.83 & 0.83 & 0.71 & 0.01 & [0,0.01] \\ \hline
    ACC & 0.73 & 0.83 & 0.85 & 0.75 & 0.00 & [0,0.01] \\ \hline
    Brier Score & 0.17 & 0.12 & 0.11 & 0.17 & 0.00 & [0,0] \\ \hline
    FN/FP Ratio & 27.67 & 2.69 & 3.04 & 1.37 & 160.58 & [35.14,1944.16] \\ \hline
    Avg Pred Prob & 0.37 & 0.37 & 0.41 & 0.52 & 0.01 & [0,0.01] \\ \hline
    \end{tabular}
    \end{subtable}
    
    \begin{subtable}{\textwidth}
    \centering
    \caption{Generalized Entropy Index}
    \begin{tabular}{|l|l|l|l|l|l|l|}
    \hline
    Metric & Group 1 & Group 2 & Group 3 & Group 4 & Generalized\_Entropy\_Index & 95\% CI \\ \hline
    TPR & 0.37 & 0.65 & 0.73 & 0.73 & 0.03 & [0.02,0.04] \\ \hline
    FPR & 0.02 & 0.13 & 0.09 & 0.20 & 0.18 & [0.1,0.28] \\ \hline
    PPR & 0.16 & 0.27 & 0.34 & 0.49 & 0.07 & [0.05,0.1] \\ \hline
    PPV & 0.94 & 0.83 & 0.89 & 0.79 & 0.00 & [0,0] \\ \hline
    NPV & 0.69 & 0.83 & 0.83 & 0.71 & 0.00 & [0,0.01] \\ \hline
    ACC & 0.73 & 0.83 & 0.85 & 0.75 & 0.00 & [0,0] \\
    Brier Score & 0.17 & 0.12 & 0.11 & 0.17 & 0.02 & [0.01,0.03] \\ \hline
    FN/FP Ratio & 27.67 & 2.69 & 3.04 & 1.37 & 0.80 & [0.45,1.24] \\ \hline
    Avg Pred Prob & 0.37 & 0.37 & 0.41 & 0.52 & 0.01 & [0.01,0.02] \\ \hline
    \end{tabular}
    \end{subtable}
\end{table}
\fi
\newpage


\section{CAUSAL DEFINITIONS OF FAIRNESS}

\subsection*{Notation}
For notions of fairness using causal reasoning, directed acyclic graphs (DAGs) are used. Let $G'=(V,E)$ be a graph with a set of nodes, $V$, and a set of directed edges, $E$. Let the nodes represent $\bf{X}$, the attributes of a patient, and the edges represent the relationship between the given attributes. These edges can be used to understand the causal impact an attribute has on the decision being made \cite{castelnovo_clarification_2022}. While we are not able to test causal definitions of fairness with an existing classifier, causal graphs can be used to initially build fair classifiers and ML algorithms \cite{verma_fairness_2018}. These causal graphs require thorough domain knowledge to understand the relationships and implications between attributes and the decision. They can then be used to further explore how social goals are being attained using a mathematical framework. For example, medical practitioners or policymakers can use the DAG to determine if a causal pathway from a sensitive attribute is admissible or problematic. We demonstrate the notions of fairness through causal definitions with a simple graph using the phenotyping example. Our graph includes our protected attribute ($G$), age, number of pre-existing conditions,  number of doctor visits in the last year and the predicted outcome of having a kidney disease or not ($D$). In causal graphs, there are proxy and resolving attributes. A proxy attribute can be used to derive another attribute while a resolving attribute is influenced by the protected attribute in a non-discriminatory way \cite{verma_fairness_2018, kilbertus_avoiding_2017}. In our scenario, a proxy attribute for race could be the number of doctor visits in the last year; access to medical care can vary based on race due to barriers including socioeconomic status, insurance status, trust in the healthcare system, etc. Using the graph in Figure \ref{figure:dag}, we define several notions of fairness in the context of our phenotyping scenario.

\begin{figure}[hbt!]
    \centering
    \includegraphics[scale = 0.5]{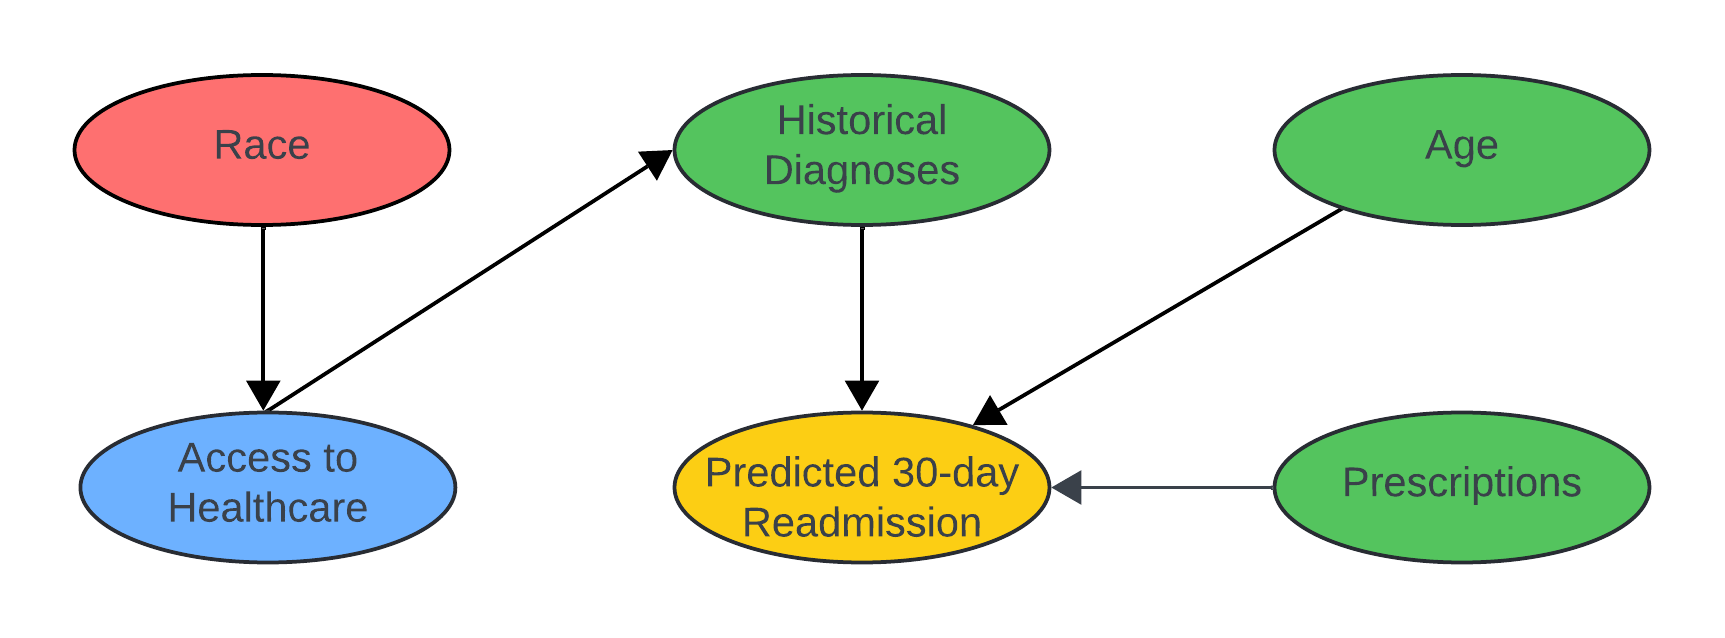}
    \caption{A causal DAG illustrating a hypothetical process for classifying a disease in patients. The DAG shows the different paths from the patient data to classification of disease through sensitive and non-sensitive attributes.}
    \label{figure:dag}
\end{figure}

\subsection*{Counterfactual Fairness}
In terms of Figure \ref{figure:dag}, counterfactual fairness would mean that our classification of the disease does not depend on any attribute that is dependent on the protected attribute $G$ \cite{verma_fairness_2018, mitchell_algorithmic_2021}. In our graph, we have that the classification of a disease is impacted by the number of doctor visits which is a descendent of race; hence, this would not be counterfactually fair. Intuitively, this would mean that if we had a White patient with $\bf{X}=\bf{x_0}$ and only counterfactually altered their race, we would expect them to have the same probability of being classified as having the disease \cite{castelnovo_clarification_2022, nilforoshan_causal_2022}.

\subsection*{No unresolved discrimination}
No unresolved discrimination is satisfied if a causal graph has no discriminatory paths from our sensitive attribute, $G$, to the classification of disease \cite{verma_fairness_2018}. A path through a resolved attribute would thus be acceptable since it is influenced in a non-discriminatory manner \cite{castelnovo_clarification_2022}. In Figure \ref{figure:dag}, we have a path from race to number of doctor visits to our classification where number of doctor visits is not a resolving attribute; thus, we have unresolved discrimination. 

\subsection*{No proxy discrimination}
A causal graph exhibits no proxy discrimination if there is no path from the sensitive attribute, $G$, to our classification of disease $D$, through a proxy \cite{verma_fairness_2018}. Using the same example of the path from race to the number of doctor visits to our classification of disease, since we have number of doctor visits as a proxy, Figure \ref{figure:dag} is not free of proxy discrimination. 

\subsection*{Fair inference}
Fair inference considers different paths to determine if they are acceptable or not \cite{verma_fairness_2018}. This requires domain knowledge of the impacts attributes have on one another and on the decision variable. For example, the number of doctor visits could be an indicator of repeated health problems. Although a proxy for race, it could be useful in determining if a patient has a disease and thus could be considered legitimate. After considering each path and classifying it as legitimate or not, a causal graph satisfies fair inference if there are no illegitimate paths from $G$ to $D$. In our case, we do not have any illegitimate paths so Figure \ref{figure:dag} satisfies fair inference. \\

Causal definitions of fairness allow us to take into consideration influences based on the sensitive attribute that may unjustly affect the final decision. This can then be used prior to building the model to determine methods to reduce these disparities so decision-making is more fair. 
%\author[1]{Jianhui Gao}
%\author[1]{Benson Chou}
%\author[2]{Zachary R. McCaw}
%\author[3]{Chuan Hong}
%\author[4]{Paul Varghese}
%\author[5]{Hilary Thurston}
%\author[1,6,7]{Jessica Gronsbell}

%\affil[1]{Department of Statistical Sciences, University of Toronto, Toronto, ON, Canada}
%\affil[2]{Department of Biostatistics, Harvard T.H.\ Chan School of Public Health, Boston, MA, USA}
%\affil[3]{Department of Biostatistics, Duke University Raleigh, NC, USA}
%\affil[4]{Verily Life Sciences, Cambridge, MA, USA}
%\affil[5]{Department of Gender \& Sexuality Studies, York University, Toronto, ON, Canada}
%\affil[6]{Department of Family \& Community Medicine, University of Toronto, Toronto, ON, Canada}
%\affil[7]{Department of Computer Science, University of Toronto, Toronto, ON, Canada}https://dl.acm.org/doi/pdf/10.1145/3514221.3517841
